# Supplementary material for: Augmenting Neural Networks with First-order Logic
Source: arXiv:1906.06298 source file (2020-08-19)
Supplement: Supplementary file 1 [file appendix.tex]

\section{Appendices}
\label{sec:appendix}

\paragraph{Setup for Machine Comprehension}
The SQuAD (v1.1.) dataset consists of $87,599$ training instances and $10,570$ development examples.
Firstly, for a specific percentage in Table~\ref{tab:mc}, we sample from the original train set.
Then we split the sampled set into 9/1 folds for training and development.
The original development set is reserved for testing only.

In our implementation of the BiDAF, we adopt Adam~\cite{paszke2017automatic} with learning rate $0.001$ for $20$ epochs.
Input word embeddings are GloVe~\cite{pennington2014glove} 300d vectors while the hidden size of each direction of BiLSTM encoder is $100$.
For the rest hyperparameters, we use the same as BiDAF. Unlike the original BiDAF, we evaluate the best model across different epochs instead of the exponential moving average one.

In our development experiments, we found the scaling term $\rho=8$ (in Equation~\ref{eq:constrained-neural-layer}) achieved the best results among all percentages.

\paragraph{Setup for Natural Language Inference}
We use Stanford Natural Language Inference (SNLI) dataset which has $549,367$ training, $9,842$ development, and $9,824$ testing examples.
For each of the percentages in Table~\ref{tab:nli}, we sample corresponding proportion from the orginal train set for training
and from the original development set for validation.
To have reliable model selection, we limit the minimal number of development examples being sampled to be $1000$.
The original test set is only for reporting.

In our implimentation of the Decomposable Attention (DAtt) model,
  we use Adam~\cite{paszke2017automatic} with learning rate $0.0001$ for $200$ epochs.
Word embeddings are 300 dimentional from GloVe~\cite{pennington2014glove}.
For the rest hyperparameters, we adopt the same setting as~\citet{parikh2016decomposable}.

We set different scaling factors (in Equation~\ref{eq:constrained-neural-layer}) for different statements.
In development experiments, we found for percentage 1 and 2, $\rho=16$ performed strongly for statement $T_1$ and $T_2$,
  while $\rho=8$ with higher percentages.
For statement $T_{3}$, we use $\rho=1$ across all percentages.

\paragraph{Setup for Text Chunking}
The CONLL2000 dataset consists of $8,936$ examples for training and $2,012$ for testing.
From the original training set, both of our training and development examples in Table~\ref{tab:tc} are sampled and split (by 9/1 folds).
Performances are then reported on the test set.

In our implementation, we set hidden size to $100$ for each direction of BiLSTM encoder.
Input word embeddings are $300$ dimentional GloVe~\cite{pennington2014glove} vectors.
Before the final linear layer, we add a dropout layer~\cite{srivastava2014dropout} with probability $0.5$
for regularization. The learning algorithm is Adam~\cite{paszke2017automatic} with learning rate $0.0001$ for $100$ epochs.

Again, we use different scaling factors (in Equation~\ref{eq:constrained-neural-layer}) for different statements.
For statements $T_{1-4}$, we found $\rho=8$ worked the best in development experiments, while
$\rho=16$ for the statements $T_{5-6}$.
The same scaling term is applied across different percentages for each statement.
